# Supplementary material for: Mixels: Fabricating Interfaces using Programmable Magnetic Pixels
Source: arXiv:2208.03804 source file (2022-08-07)
Supplement: Supplementary file 1 [file 11-additional-material.tex]

The primary requirements of any magnetic plotter are its ability to become strongly polarized (to program strong magnetic pixels), to be able to program pixels of a desired size (to achieve the resolution required of the applications), and to easily turn off (to save power and prevent interference with other electronics in a fabrication system). Besides the common goal of high magnetic strength, the key requirements of a programmable magnetic surface is to be able hold a programmed magnetic pattern even when the plotter is removed (so that it can be used indefinitely as a passive interactive device), and to be able to turned "off" magnetically in order to not be constrained to always interacting repulsively or attractively to another magnetic surface.

\subsection{Magnetic Sheet Material}

We chose a medium-soft magnetic sheet material (type: inexpensive ferromagnetic material (fridge magnet), thickness: XXmm) for our system. We chose a medium-soft magnetic material because softer magnetic materials are easier reprogrammable than harder magnetic materials. One reason for this is that soft magnetic materials exhibit high \textit{permeability}, i.e. they need weaker electromagnets to reach a certain magnetic strength. In addition, soft magnetic materials are easier to reset because they exhibit lower \textit{coercity}, which is a magnetic property that describes how easily a magnetic material gets demagnetized under a magnetic field. However, as a drawback soft magnetic materials exhibit lower \textit{saturation} and thus have less magnetic strength. In addition, since magnetic materials lose magnetic strength when removed from the electromagnet, softer magnetic materials have less magnetic strength after removal, a property called \textit{remanence}, since they start from a lower saturation. We provide a characterization of the different magnetic properties for our chosen sheet material in section 'Evaluation'.

% because the saturation of soft magnetic materials is low, they 

% they tend to lose more magnetization when removed from the electromagnet because they exhibit lower \textit{remanence}, a magnetic property that describes how well a magnetic material keeps its magnetic strength.

% High permeability and maximum flux density (saturation) are typically desirable for both magnetically soft and hard materials, though uncommon in the former. However saturation, coercivity and remanence typically correlate and depend on the hardness of the magnetic material: hard magnetic materials exhibit high saturation, coercivity and remanence, and are thus difficult to change, making them ideal candidates for permanent magnets but less suitable a sheet that should be easily programmable. We therefore chose to utilize a medium-soft material for our magnetic sheet that exhibits high permeability. The remanence of such material will make it \textit{programmable} by retaining a magnetic pattern programmed into it, but its low saturation will maintain its ability to be \textit{re-programmable} with a modest external field. Though a harder material sheet would be stronger magnetically, our research thus aims to illustrate how 2D plotting and reading can be utilized with these magnetic insights to develop new use cases, above building an optimized setup. In contrast to hard magnetic materials, those said to be magnetically "soft" exhibit low magnetic saturation, coercivity and remanence; these are easy to magnetize and are typified by electromagnets.

\subsection{Electromagnet}

We chose an electromagnet over a permanent magnet because electromagnets their polarity can be reversed digitally by changing the direction of current applied through it. In addition, electromagnets allow us to continuously vary the magnetic strength of each pixel by regulating the magnitude of current through them~\cite{yasu2020magnelayer,yasu2017magnetic}. 

However, as a drawback, electromagnets of the same diameter as permanent magnets exhibit less magnetic strength. Thus, the resulting magnetic pixels have less magnetic strength. To create magnetic pixels of the same resolution and strength when using an electromagnet, we therefore shape the electromagnet into a cone shape that becomes wider above the magnetic sheet and that concentrates the magnetic flux at the tip of the electromagnet. As a result, our shaped electromagnet for a certain pixel size creates a stronger magnetic pixel than a permanent magnet for the same pixel size. 

% When choosing an electromagnet, our goal was to choose one that allows us to magnetize the sheet to full saturation. In addition, we use a highly permeable core to safe power when creating the magnetic field. 

\subsection{Magnetization - Demagnetization Cycle}

\textbf{Magnetization:} We start by inserting the sheet into the magnetic plotter. At the beginning, the sheet is fully demagnetized. We then turn on the electromagnet, which is polarized, e.g. in the north direction. This increases the magnetic sheet's strength until maximum saturation. We then turn off the electromagnet. 

\textbf{Remaining Magnetized:} With the electromagnet turned off, the strength of the magnetic sheet drops only marginally, i.e. retains a significant portion of its magnetic strength. This is because soft magnetic materials exhibit high remanescence. 

\textbf{Demagnetization:} To demagnetize the soft magnetic sheet, we then turn on the electromagnet in the opposite direction, e.g. in the south direction. As we increase the strength of the electromagnet in the south direction, the strength of the magnetic sheet decreases in that polarity. We continue to do this until the sheet becomes magnetically neutral. The strength of the electromagnetic required to fully demagnetize the sheet is called coercivity.

% \vspace{5pt}
% \noindent\textbf{Properties of Magnetic Materials:} Key to these requirements are the magnetic attributes of magnetic flux density, saturation, permeability, coercivity, and remanence. Magnetic flux density (known as the B field) is a measure of the actual magnetic field strength of an object or material, and saturation refers to a material's upper bound of this density. When a ferromagnetic object is placed in an external magnetic field (known in this context as the H field), the object's magnetic dipoles will tend to align with the direction of the external magnetic field, increasing the objects magnetic flux density and making it stronger. Magnetic permeability ($\mu$) describes the degree to which the material's magnetic flux density changes given a change in the strength of a surrounding magnetic field; graphically speaking, it is the slope of the B-H curve (Figure \ref{fig:BH-emag}), exhibiting the relation $B=\mu(H)H$. Once magnetized, materials with high remanence will retain a significant fraction of their magnetization even when removed from the external field; a low-remanence material will not. Similarly, if a material has low coercivity, it is easily demagnetized when placed in an external magnetic field, whereas high coercivity material is not.  

\subsection{Attraction, Repulsion, Agnosticism}

Magnetic surfaces can either attract, repulse, or be agnostic, i.e. not attract or repulse other magnetic surfaces. If two surfaces are plotted with oppositely polarized magnetic pixels, those surfaces will attract; if the polarized magnetic pixels are plotted with identical polarities, they will repel.

There are two ways to achieve agnosticism, either through demagnetization or through a set of attractive or repulsive pixels that cancel each other. Demagnetization works only if both surfaces are demagnetized. If one surface is demagnetized while the other is magnetized (in any polarization), the magnetized surface may coerce the demagnetized surface into attraction (this is why nails do not nominally attract other nails, but as ferromagnetic objects they will nonetheless be coerced to attract magnets). Thus, to create agnosticism even if one surface is magnetized, sets of attractive or repulsive pixels...

The last requirement for magnetic surface stated above is to allow selective attraction to only particular surfaces,

To achieve selectivity and agnosticism, we leverage our ability to plot arbitrary 2D patterns to program matrices with rows and columns whose binary-valued elements (1 or -1) we design to be mutually orthogonal (Figure \ref{fig:theory-predict}). Such matrices are known as Hadamard matrices. Magnetically speaking, two surfaces with like elements overlapping will repel, and unlike elements will attract. However, because the dot product between two orthogonal vectors is 0, when two surfaces programmed with our row- and column-orthogonal matrices are superimposed, the locally attractive and repulsive pixel interactions cancel exactly to create a globally agnostic interface. At the same time, if the two matrices chosen are with identical or opposite, there will exist a single position in which all pixels on the surfaces will be perfectly repulsive or attractive, respectively.  
